# Supplementary material for: Towards Self-Contained Answers: Entity-Based Answer Rewriting in Conversational Search
Source: arXiv:2403.01747 source file (2024-03-04)
Supplement: Supplementary file 1 [file chiir2024-appendix.tex]

\appendix

\section{Examples of answer rewrites}
\label{sec:appendix_rewrites}

Table \ref{tbl:rewrites} shows several examples of answer rewrites.

\begin{table*}[]
\caption{Examples of different answer rewrites.}
\label{tbl:rewrites}
\resizebox{\textwidth}{!}{%
\begin{tabular}{llll}
\toprule
question & A-original & A-inlinedef & A-followup \\
\midrule
\begin{tabular}[c]{@{}l@{}}where does harry potter\\  get his school supplies?\end{tabular} & \begin{tabular}[c]{@{}l@{}}Hagrid explains that Harry Potter will buy what he\\  needs for school in Diagon Alley.\end{tabular} & \begin{tabular}[c]{@{}l@{}}Hagrid (fictional character from Harry Potter) explains that \\ Harry Potter (fantasy literature series by J.K. Rowling) \\ will buy what he needs for school in Diagon Alley\\  (places mentioned in Harry Potter).\end{tabular} &  \begin{tabular}[c]{@{}l@{}}Hagrid explains that Harry Potter will buy what he needs\\  for school in Diagon Alley. If you would like to learn more\\  about Harry Potter, Rubeus Hagrid or places in Harry\\  Potter, feel free to ask!\end{tabular} \\
\midrule
\begin{tabular}[c]{@{}l@{}}What are the main uses\\  of solar energy?\end{tabular} &  \begin{tabular}[c]{@{}l@{}}Solar energy is used today in a number of ways: As heat for\\  making hot water, heating buildings, and cooking. To generate\\  electricity with solar cells or heat engines. To take the salt\\  away from sea water. To use sun rays for drying clothes and\\  towels. It is used by plants for the process of photosynthesis.\end{tabular} & \begin{tabular}[c]{@{}l@{}}Solar energy is used today in a number of ways: As heat for\\  making hot water, heating buildings, and cooking. To generate\\  electricity with solar cells or heat engines.To take the salt away\\  from sea water.To use sun rays (electromagnetic radiation\\  given off by the Sun) for drying clothes and towels. It is used \\ by plants for the process of photosynthesis.\end{tabular} &\begin{tabular}[c]{@{}l@{}}Solar energy is used today in a number of ways: As heat\\  for making hot water, heating buildings, and cooking. \\ To generate electricity with solar cells or heat engines.\\ To take the salt away from sea water. To use sun rays\\  for drying clothes and towels.It is used by plants for\\  the process of photosynthesis. If you would\\  like to learn more about sunlight, feel free to ask!\end{tabular} \\
\midrule
\begin{tabular}[c]{@{}l@{}}Why was Sisyphus punished\\  to push the rock up the hill?\end{tabular} & \begin{tabular}[c]{@{}l@{}}Sisyphus was punished for his self-aggrandizing \\ craftiness and deceitfulness.\end{tabular} & \begin{tabular}[c]{@{}l@{}}Sisyphus, who was the king of Ephyra in Greek mythology, \\ was punished for his self-aggrandizing craftiness and deceitfulness.\end{tabular} & \begin{tabular}[c]{@{}l@{}}Sisyphus was punished for his self-aggrandizing craftiness and \\ deceitfulness. Would you like to learn more about Sisyphus?\end{tabular} \\
\midrule
\begin{tabular}[c]{@{}l@{}}where do you find dwellings made of ice\\  who makes them and what are they called?\end{tabular} & \begin{tabular}[c]{@{}l@{}}An igloo is a type of shelter built of snow, often \\ associated with Inuit, Eskimo peoples, and people \\ of Canadas Central Arctic and Greenlands Thule area.\end{tabular} & \begin{tabular}[c]{@{}l@{}}An igloo is a type of shelter, referring to shallow cave-like\\  opening at the base of a bluff or cliff, built of snow, often\\  associated with Inuit, Eskimo peoples, and people of \\ Canadas Central Arctic and Greenlands, an autonomous\\  country within the Kingdom of Denmark on world's \\ largest island, Thule area.\end{tabular} & \begin{tabular}[c]{@{}l@{}}An igloo is a type of shelter built of snow, often associated \\ with Inuit, Eskimo peoples, and people of Canadas Central \\ Arctic and Greenlands Thule area. Would you like to \\ learn more about Greenland or shelter?\end{tabular} \\
\midrule
who introduced four c model of creativity? & \begin{tabular}[c]{@{}l@{}}James C. Kaufman and Beghetto introduced a four \\ C model of creativity.\end{tabular} & \begin{tabular}[c]{@{}l@{}}James C. Kaufman, an American psychologist, and Beghetto\\  introduced a four C model of creativity.\end{tabular} & \begin{tabular}[c]{@{}l@{}}James C. Kaufman and Beghetto introduced a four C model of creativity. \\ Would you like to learn more about James C. Kaufman?\end{tabular} \\
\midrule
Tell me about the phospholipid bilayer. & \begin{tabular}[c]{@{}l@{}}The lipid bilayer is a thin polar membrane made of two layers\\  of lipid molecules. These membranes are flat sheets that form\\  a continuous barrier around all cells.\end{tabular} & \begin{tabular}[c]{@{}l@{}}The lipid bilayer is a thin polar membrane made of two layers\\  of lipid molecules, which are a class of nonpolar substances\\  of either biological or artificial origin. These membranes are\\  flat sheets that form a continuous barrier, an energy that \\ must be input to a system to undergo a process, around all\\  cells, which are basic structural and functional unit \\ of all organisms.\end{tabular} & \begin{tabular}[c]{@{}l@{}}The lipid bilayer is a thin polar membrane made of two layers of lipid molecules. \\ These membranes are flat sheets that form a continuous barrier around all cells. \\ Would you like to learn more about Activation energy, Cell (biology) or Lipid?\end{tabular} \\
\midrule
\begin{tabular}[c]{@{}l@{}}Who crossed the alps and invaded italy\\  with an army of elephants during the \\ second punic war?\end{tabular} & \begin{tabular}[c]{@{}l@{}}Hannibal made his famous military exploit of carrying war to\\  Italy by crossing the Alps with his African elephants.\end{tabular} & \begin{tabular}[c]{@{}l@{}}Hannibal, a Carthaginian general during the Second Punic War\\  with the Roman Republic, made his famous military exploit \\ of carrying war to Italy by crossing the Alps with his African, \\ which is a continent on the Earth, elephants.\end{tabular} & \begin{tabular}[c]{@{}l@{}}Hannibal made his famous military exploit of carrying war to Italy by \\ crossing the Alps with his African elephants. If you would like to learn\\  more about Africa or Hannibal, feel free to ask!\end{tabular}
\\ \bottomrule
\end{tabular}
}
\end{table*}

\section{A sample of gathered feedback data on answer rewrite types}
\label{sec:appendix_reasons}
Table \ref{tbl:reasons} shows several justifications for the choice of answer rewrite type, as reported by crowd workers.

\begin{table*}[]
\caption{Analysis of reasons provided by the crowd workers on why they prefer certain answer.}
\label{tbl:reasons}
%\resizebox{\textwidth}{!}{%
\begin{tabular}{ll}
\toprule
Answer chosen & Reason provided \\
\midrule
\multirow{4}{*}{\emph{A-original}} & - I chose it because it gave the necessary information without adding unnecessary text. \\
 & - contains the answer without any extra details. short and to the point. \\
 & \begin{tabular}[c]{@{}l@{}} - The most concise answer. I don't think the recipient would want any more particular\\  information especially about Africa\end{tabular} \\
 & - It is simple and to the point \\
 \midrule
\multirow{4}{*}{\emph{A-inlinedef}} & - explains what data is and doesn't add the unnecessary "feel free to ask". \\
 & - I think this is the best answer and explains everything in an easy to understand way. \\
 & \begin{tabular}[c]{@{}l@{}}- They're all sort of the same, but I feel this one goes out of its way to define other\\  phrases that might not be understood otherwise (cultural movement and visual artworks),\\  so it is the most comprehensive.\end{tabular} \\
 \midrule
 & - The Answer\_1 explain about the lipid bilayer clearly comparatively to other answers \\
\multirow{4}{*}{\emph{A-followup}} & \begin{tabular}[c]{@{}l@{}}- It gives the most info without assuming the recipient isn't intelligent while encouraging\\  them to engage further to ask for more details.\end{tabular} \\
 & \begin{tabular}[c]{@{}l@{}}- I chose option 2 because not only did it answer the question but it included an open ended\\  option for the person receiving the information, to ask more questions if they wanted.\end{tabular} \\
 & I want to know more about mood psychology. \\
 & \begin{tabular}[c]{@{}l@{}}- I like that the answer doesn't assume that I don't know that the Houston Astros are a \\ baseball team, but offers to get me more info about them if I want it.\end{tabular}
 \\ \bottomrule
\end{tabular}%
%}
\end{table*}
